# Supplementary material for: A Model-Based Approach to Imitation Learning through Multi-Step Predictions
Source: arXiv:2504.13413 source file (2025-04-18)
Supplement: Supplementary file 1 [file A1-appendix-0125.tex]

\section{}

In this section, we show a sample complexity bound for the proposed algorithm in linear systems.

\subsection{Settings and Our Algorithm}

The dynamics of the \emph{known} linear time-invariant (LTI) system is specified by
\begin{equation*}
  x_{t+1} = Ax_t + Bu_t,
\end{equation*}
and the objective is to imitate the expert controller $\pi^{\exp}(x_t) = K^{\exp} x_t$ by a linear feedback controller
\begin{equation*}
  u_t = \pi(x_t) = K x_t.
\end{equation*}The observation of states and control inputs is subject to measurement noise
\begin{align*}
  y_t &= x_t + \xi_t,\\
  v_t &= u_t + \eta_t.
\end{align*}
The objective is to learn a controller $\hat{K}$ from the data $(y_{1:T}, v_{1:T})$ that minimizes the error $\norm{\hat{K} - K^{\exp}}$. We will make heavy use of the $\tau$-step transition matrix $x_{t+\tau} = G^{\star}_{\tau} x_t$, where the ground truth is given by $G^{\star}_{\tau} = A_K^{\tau}$.

The proposed algorithm now becomes the following:
\begin{equation}
  \min_{K, G_{1:H}}\quad \sum_{t=0}^{T-H} \sum_{\tau=1}^{H} \norm{y_{t+\tau} - G_{\tau} y_t}_Q^2 + \norm{v_{t+\tau-1} - K G_{\tau-1} y_t}_R^2 + \norm{G_{\tau} y_t - (A+BK) G_{\tau-1} y_t}_P^2.
\end{equation}


\subsection{The Optimal Solution}
We compare the aforementioned optimal solution $\hat{K}$ to the following benchmark controller $\hat{K}^{\bmk}$
\begin{equation}
    \hat{K}^{\bmk} = \mathop{\arg\min}_{K} \sum_{t=0}^{T-H} \norm{v_t - Ky_t}^2 = \sum_t v_ty_t^\top \Bigl(\sum_t y_ty_t^\top\Bigr)^{-1}
\end{equation}

\begin{lemma}
  $\nabla_{A} \tr(A^{\top} B) = \nabla_{A} \tr(B^{\top} A) = B$.
\end{lemma}


\begin{lemma}
  $\nabla_{A} \tr(CABA^{\top}) = CAB + C^{\top} A B^{\top}$.
\end{lemma}

\begin{proof}
  
\end{proof}


\begin{lemma}
  $\nabla_{A} \norm{(M+NA) x - b}_R^2 = 2N^{\top} R \bigl( (M+NA)x - b \bigr) x^{\top}$.
\end{lemma}

\begin{proof}
  By direct calculation we have
  \begin{subequations}
  \begin{align}
    & \nabla_{A} \norm{(M+NA) x - b}_R^2 \\
    ={}& \nabla_{A} \tr(((M+NA) x - b)^{\top} R ((M+NA) x - b)) \\
    ={}& \nabla_{A} \tr(R ((M+NA) x - b) ((M+NA) x - b)^{\top}) \\
    ={}& \nabla_{A} \tr(R (M+NA) xx^{\top} (M+NA)^{\top} - Rb x^{\top} (M+NA)^{\top} - R(M+NA)x b^{\top} ) \\
    ={}& \nabla_{A} \tr( R NA xx^{\top} A^{\top} N^{\top} + 2RMxx^{\top} A^{\top} N^{\top} - 2Rb x^{\top} A^{\top} N^{\top}) \\
    ={}& \nabla_A{} \tr( 2N^{\top} R(Mx-b) x^{\top} A^{\top} + N^{\top} RNAxx^{\top} A^{\top} ) \\\
    ={}& 2 N^{\top} R (Mx-b) x^{\top} + 2 (N^{\top} RN) A (xx^{\top}) \\
    ={}& 2 N^{\top} R ((M+NA)x - b) x^{\top}.
  \end{align}
  \end{subequations}
\end{proof}


\begin{theorem}
  The optimal solution is given by
  \begin{align}
    K &= -(R + B^{\top} P B)^{-1} \left( \sum_{t,\tau} (B^{\top} PA G_{\tau-1} y_t - R v_{t+\tau-1} - B^{\top} P G_{\tau} y_t) (G_{\tau-1} y_t)^{\top} \right) \left( \sum_{t,\tau} (G_{\tau-1} y_t) (G_{\tau-1} y_t)^{\top} \right)^{-1} \\
    &= (R + B^{\top} P B)^{-1} \left( \sum_{t,\tau} (B^{\top} P BK^{\star} G_{\tau-1} y_t + R v_{t+\tau-1}) (G_{\tau-1} y_t)^{\top} \right) \left( \sum_{t,\tau} (G_{\tau-1} y_t) (G_{\tau-1} y_t)^{\top} \right)^{-1} \\
    &= K^{\star} + (R + B^{\top} P B)^{-1} \left( \sum_{t,\tau} R(\eta_t - K^{\star} G_{\tau-1} \xi_t) (G_{\tau-1} y_t)^{\top} \right) \left( \sum_{t,\tau} (G_{\tau-1} y_t) (G_{\tau-1} y_t)^{\top} \right)^{-1}
  \end{align}
\end{theorem}


\newpage
\section{Obsolete}

In this section, we show a sample complexity bound for the proposed algorithm in linear systems.

\subsection{Settings and Our Algorithm}

The dynamics of the \emph{known} linear system is specified by
\begin{equation*}
  x_{t+1} = Ax_t + Bu_t,
\end{equation*}
and the objective is to imitate the expert controller $\pi^{\exp}(x_t) = K^{\exp} x_t$ by a linear feedback controller
\begin{equation*}
  u_t = \pi(x_t) = K x_t.
\end{equation*}
The observation of states and control inputs is subject to measurement noise
\begin{align*}
  y_t &= x_t + \xi_t,\\
  v_t &= u_t + \eta_t.
\end{align*}
The objective is to learn a controller $\hat{K}$ from the data $(y_{1:T}, v_{1:T})$ that minimizes the error $\norm{\hat{K} - K^{\star}}$. We will make heavy use of the $\tau$-step transition matrix $x_{t+\tau} = G^{\star}_{\tau} x_t$, where the ground truth is given by $G^{\star}_{\tau} = A_K^{\tau}$.

The proposed algorithm now becomes the following.

\begin{algorithm}[H]
  \caption{Our algorithm in linear systems}
  \begin{algorithmic}[1]
    \State Use ordinary least-squares (OLS) to recover $\tau$-step transition matrices:
    \begin{equation*}
      \hat{G}_{\tau} \gets \arg\min_{G_{\tau}} \sum_{t=1}^{T} \norm{y_{t+\tau} - G_{\tau} y_t}^2,\quad \forall \tau \in [m].
    \end{equation*}
    \State Recover the controller by \textcolor{red}{[This may be inconsistent with the generic algorithm.]}
    \begin{equation*}
      \hat{K} \gets \arg\min_{K} \sum_{\tau=1}^{m} \norm{\hat{G}_{\tau+1} - A_K \hat{G}_{\tau}}^2.
    \end{equation*}
  \end{algorithmic}
\end{algorithm}

\subsection{Sample Complexity}

We proceed to analyze the sample complexity of the algorithm.

\paragraph{Stage 1.} Denote the objective of the first stage by
\begin{equation}
  \L_1 := \sum_{t=1}^{T} \norm{y_{t+\tau} - G_{\tau} y_t}^2.
\end{equation}
Note that the first-order criterion dictates that
\begin{equation}
  \left. \frac{\partial \L_1}{\partial G_{\tau}} \right\vert_{\hat{G}_{\tau}} = 2 \sum_{t=1}^{T} (y_{t+\tau} - \hat{G}_{\tau} y_t) y_t^{\top} = 0,
\end{equation}
or equivalently,
\begin{equation}
  \hat{G}_{\tau} \sum_{t=1}^{T} y_t y_t^{\top}
  = \sum_{t=1}^{T} y_{t+\tau} y_t^{\top}
  = \sum_{t=1}^{T} \prn[\big]{ G^{\star}_{\tau}(y_t - \xi_t) + \xi_{t+\tau} } y_t^{\top} y_t^{\top}
  = G^{\star}_{\tau} \sum_{t=1}^{T} y_t y_t^{\top} + \sum_{t=1}^{T} (\xi_{t+\tau} - G^{\star}_{\tau} \xi_t) y_t^{\top}.
\end{equation}
Therefore, assuming invertibility of $\hSigma_y := \frac{1}{T} \sum_{t=1}^{T} y_t y_t^{\top}$, we have
\begin{equation}
  \hat{G}_{\tau} = G^{\star}_{\tau} + \prn*{ \sum_{t=1}^{T} (\xi_{t+\tau} - G^{\star}_{\tau} \xi_t) y_t^{\top} } \prn*{ \sum_{t=1}^{T} y_t y_t^{\top} }^{-1}
  = G^{\star}_{\tau} + \frac{1}{T} \prn*{ \sum_{t=1}^{T} (\xi_{t+\tau} - G^{\star}_{\tau} \xi_t) y_t^{\top} } \hSigma_y^{-1}.
\end{equation}
Note that
\begin{align}
  \Es{\hSigma_y}
  &= \E{\frac{1}{T} \sum_{t=1}^{T} (x_t+\xi_t) (x_t+\xi_t)^{\top}} \\
  &= \frac{1}{T} \brak*{ \sum_{t=1}^{T} \E{x_t x_t^{\top}} + \sum_{t=1}^{T} \E{x_t \xi_t^{\top} + \xi_t x_t^{\top}} + \sum_{t=1}^{T} \E{\xi_t \xi_t^{\top}} } \\
  &= \frac{1}{T} \sum_{t=1}^{T} x_t x_t^{\top} + \varSigma_{\xi}
  \succeq \varSigma_{\xi}.
\end{align}
Finally, by concentration inequality we have, with high probability,
\begin{equation}
  \hSigma_y \succeq \frac{1}{2} \varSigma_{\xi}.
\end{equation}
For the other factor in the residue term, we assume that $\xi_t \sim \mathcal{N}(\zero, \varSigma_{\xi})$, such that
\begin{equation}
  \sum_{t=1}^{T} (\xi_{t+\tau} - G^{\star}_{\tau} \xi_t) y_t^{\top}
\end{equation}

\subsection{Experimental Details \& Results Tables \& Environment Pictures}
